# Supplementary material for: Popularity Bias in Recommendation: A Multi-stakeholder Perspective
Source: arXiv:2008.08551 source file (2020-08-19)
Supplement: Supplementary file 1 [file appendixA.tex]

\chapter{Weird Exam Answers}	% *NOT* \OnePageChapter

\paragraph{About appendices:}
	Each appendix follow the same page-numbering rules
	as a regular chapter; the first page of a
	(multi-page) appendix is not numbered.
	By the way, the following are supposedly
	authentic answers to English GCSE exams!

\begin{enumerate}

\item
The Greeks were a highly sculptured people, and without
them we wouldnt have history. The Greeks also had myths.
A myth is a female moth.

\item
Actually, Homer was not written by Homer but by another
man of that name.

\item
Socrates was a famous Greek teacher who went around
giving people advice. They killed him. Socrates died from an
overdose of wedlock. After his death, his career suffered a
dramatic decline.

\item
Julius Caesar extinguished himself on the battlefields
of Gaul. The Ides of March murdered him because they thought
he was going to be made king. Dying, he gasped out: Tee hee,
Brutus.

\item
Nero was a cruel tyranny who would torture his subjects
by playing the fiddle to them.

\item
In midevil times most people were alliterate. The
greatest writer of the futile ages was Chaucer, who
wrote many poems and verses and also wrote literature.

\item
Another story was William Tell, who shot an arrow
through an apple while standing on his sons head.

\item
Writing at the same time as Shakespeare was Miguel
Cervantes. He wrote Donkey Hote. The next great author
was John Milton. Milton wrote Paradise Lost. Then his
wife died and he wrote Paradise Regained.

\item
During the Renaissance America began. Christopher
Columbus was a great navigator who discovered America while
cursing about the Atlantic. His ships were called the Nina,
the Pinta, and the Santa Fe.

\item
Gravity was invented by Issac Walton. It is chiefly
noticeable in the autumn when the apples are falling
off the trees.

\item
Johann Bach wrote a great many musical compositions and
had a large number of children. In between he practiced on
an old spinster which he kept up in his attic. Bach died
from 1750 to the present. Bach was the most famous composer
in the world and so was Handel. Handel was half German
half Italian and half English. He was very large.

\item
Soon the Constitution of the United States was adopted
to secure domestic hostility. Under the constitution the
people enjoyed the right to keep bare arms.

\item
The sun never set on the British Empire because the
British Empire is In the East and the sun sets in the West.

\item
Louis Pasteur discovered a cure for rabbis. Charles
Darwin was a naturalist who wrote the Organ of the Species.
Madman Curie discovered radio. And Karl Marx became one of
the Marx brothers.

\end{enumerate}
