# Supplementary material for: Popularity Bias in Recommendation: A Multi-stakeholder Perspective
Source: arXiv:2008.08551 source file (2020-08-19)
Supplement: Supplementary file 2 [file appendixB.tex]

\chapter{Ode to Spot}	\OnePageChapter         % ONE PAGE!

\noindent\paragraph{(Data, Stardate 1403827)}
(A one-page chapter --- page must be numbered!)
Throughout the ages, from Keats to Giorchamo, poets have
composed ``odes'' to individuals who have had a profound effect
upon their lives.  In keeping with that tradition
I have written my next poem \ldots in honor of my cat.
I call it\ldots{}Ode\ldots{}to Spot.
(Shot of Geordi and Worf in audience,
looking mystified at each other.)

\begin{quotation}
\noindent Felus cattus, is your taxonomic nomenclature \\
an endothermic quadruped, carnivorous by nature? \\
Your visual, olfactory, and auditory senses \\
contribute to your hunting skills, and natural defenses. \\
I find myself intrigued by your sub-vocal oscillations, \\
a singular development of cat communications \\
that obviates your basic hedonistic predilection \\
for a rhythmic stroking of your fur to demonstrate affection. \\
A tail is quite essential for your acrobatic talents; \\
you would not be so agile if you lacked its counterbalance. \\
And when not being utilized to aid in locomotion, \\
It often serves to illustrate the state of your emotion.
\end{quotation}

\noindent(Commander Riker begins to applaud, until a
glance from Counselor Troi brings him to a halt.)
Commander Riker, you have anticipated my denouement.
However, the sentiment is appreciated.  I will continue.

\begin{quotation}
\noindent O Spot, the complex levels of behavior you display \\
connote a fairly well-developed cognitive array. \\
And though you are not sentient, Spot, and do not comprehend \\
I nonetheless consider you a true and valued friend.
\end{quotation}
